# Supplementary material for: Why Prompt Optimization Works, and Why It Sometimes Doesn't: A Causal-Inspired Edit-Level Analysis
Source: arXiv:2605.26655 source file (2026-05-26)
Supplement: Supplementary file 1 [file appendix.tex]

\section{Full CATE Table (All 12 Features)}
\label{sec:app_full_cate}

\begin{table}[h]
\centering
\small
\caption{Full SIPW-adjusted CATE for all 12 features. Features not shown in the main table: Politeness and Encourage\_germane\_load. $\bigstar$~$=$~BH-FDR $q < 0.05$.}
\begin{tabular}{lrrrrr}
\toprule
\textbf{Feature} & \textbf{CS} & \textbf{Math} & \textbf{Logic} & \textbf{Seq.} & \textbf{MH} \\
\midrule
Politeness & $+0.004$ & $-0.018$ & $+0.007$ & $+0.012$ & $-0.005$ \\
Enc.\ germane & $-0.012$ & $-0.033$ & $+0.021$ & $+0.028$ & $-0.016$ \\
(all others as in Table~\ref{tab:cate_main}) \\
\bottomrule
\end{tabular}
\end{table}

\section{Full Leave-One-Dataset-Out Table}
\label{sec:app_loo}

Table~\ref{tab:app_loo_full} shows per-split CATE estimates for all 18 LOO configurations.

\begin{table*}[h]
\centering
\small
\caption{Full LOO stability table. CATE\_A and CATE\_B are the IPTW-adjusted effects for the two task types in the reversal, with the indicated dataset left out. ``Stable'' = sign matches full-data baseline.}
\label{tab:app_loo_full}
\setlength{\tabcolsep}{4pt}
\begin{tabular}{llllrrl}
\toprule
\textbf{LOO Dataset} & \textbf{Feature} & \textbf{Task A} & \textbf{Task B} & \textbf{CATE\_A} & \textbf{CATE\_B} & \textbf{Stable?} \\
\midrule
CommonsenseQA & llm:Extraneous\_load & commonsense & math & $+0.026$ & $-0.150$ & \checkmark \\
causal\_judgement & llm:Extraneous\_load & commonsense & math & $+0.015$ & $-0.150$ & \checkmark \\
disambiguation\_qa & llm:Extraneous\_load & commonsense & math & $+0.053$ & $-0.150$ & \checkmark \\
GSM8K & llm:Extraneous\_load & commonsense & math & $+0.032$ & $-0.324$ & \checkmark \\
MultiArith & llm:Extraneous\_load & commonsense & math & $+0.032$ & $-0.030$ & \checkmark \\
GSM8K & llm:Demos & math & sequential & $+0.182$ & $-0.088$ & \checkmark \\
MultiArith & llm:Demos & math & sequential & $+0.083$ & $-0.088$ & \checkmark \\
GSM8K & surf:n\_demos & math & sequential & $+0.128$ & $+0.071$ & \checkmark \\
MultiArith & surf:n\_demos & math & sequential & $+0.043$ & $+0.071$ & \checkmark \\
CommonsenseQA & llm:Metacognition & sequential & commonsense & $+0.082$ & $+0.034$ & \checkmark \\
causal\_judgement & llm:Metacognition & sequential & commonsense & $+0.082$ & $+0.003$ & \checkmark \\
disambiguation\_qa & llm:Metacognition & sequential & commonsense & $+0.082$ & $-0.032$ & $\times$ \\
boolean\_expressions & surf:step\_words & logical & multihop & $+0.111$ & $+0.064$ & \checkmark \\
coin\_flip & surf:step\_words & logical & multihop & $+0.039$ & $+0.064$ & \checkmark \\
StrategyQA & surf:step\_words & logical & multihop & $+0.076$ & $+0.159$ & \checkmark \\
date\_understanding & surf:step\_words & logical & multihop & $+0.076$ & $-0.060$ & $\times$ \\
StrategyQA & surf:word\_count & sequential & multihop & $+0.027$ & $+0.159$ & \checkmark \\
date\_understanding & surf:word\_count & sequential & multihop & $+0.027$ & $-0.020$ & $\times$ \\
\midrule
\textbf{Total} & & & & & & \textbf{15/18 (83\%)} \\
\bottomrule
\end{tabular}
\end{table*}

\section{Per-Dataset Motif Effect Breakdown}
\label{sec:app_motif_breakdown}

Table~\ref{tab:app_motif} shows naive (unweighted) CATE for chain\_of\_thought and meta\_instruction insertions by dataset.
The strongest per-dataset effects are MultiArith for both motifs (chain\_of\_thought: $-0.162$; meta\_instruction: $-0.277$).
The math task-type result is partially driven by MultiArith; task-type-level conclusions should be interpreted with this heterogeneity in mind.

\begin{table}[h]
\centering
\small
\caption{Naive CATE per dataset for chain-of-thought and meta-instruction motifs.}
\label{tab:app_motif}
\begin{tabular}{llrr}
\toprule
\textbf{Motif} & \textbf{Dataset (Task)} & \textbf{CATE} & \textbf{n treated} \\
\midrule
\multirow{10}{*}{chain\_of\_thought} & boolean\_expr.\ (Logic) & $-0.034$ & 189 \\
 & coin\_flip (Logic) & $+0.088$ & 184 \\
 & GSM8K (Math) & $+0.027$ & 203 \\
 & MultiArith (Math) & $\mathbf{-0.162}$ & 139 \\
 & CommonsenseQA (CS) & $-0.024$ & 211 \\
 & causal\_judg.\ (CS) & $+0.051$ & 201 \\
 & disambiguation (CS) & $+0.031$ & 164 \\
 & last\_letters (Seq.) & $+0.067$ & 160 \\
 & StrategyQA (MH) & $+0.002$ & 152 \\
 & date\_und.\ (MH) & $+0.060$ & 206 \\
\midrule
\multirow{7}{*}{meta\_instruction} & GSM8K (Math) & $-0.019$ & 14 \\
 & MultiArith (Math) & $\mathbf{-0.277}$ & 64 \\
 & coin\_flip (Logic) & $+0.066$ & 91 \\
 & last\_letters (Seq.) & $-0.004$ & 54 \\
 & CommonsenseQA (CS) & $+0.005$ & 50 \\
 & StrategyQA (MH) & $-0.034$ & 43 \\
 & date\_und.\ (MH) & $-0.035$ & 60 \\
\bottomrule
\end{tabular}
\end{table}

\section{Conditional Independence Structure (Exploratory)}
\label{sec:app_dag}

We pool prompt observations per task type and apply the PC algorithm \cite{spirtes2000causation} (Fisher-Z test, $\alpha = 0.05$) and DirectLiNGAM \cite{shimizu2006lingam} on the 12-feature vectors.
Average cross-task Jaccard similarity~$= 0.249$, confirming substantial structural heterogeneity.
Pairwise similarity: commonsense vs.\ math~$= 0.053$; math vs.\ logical~$= 0.111$; math vs.\ multihop~$= 0.188$; commonsense vs.\ logical~$= 0.385$; logical vs.\ sequential~$= 0.667$.
Math tasks have the most distinctive conditional independence structure.
\textbf{No mechanism claims are made from these exploratory analyses.}

\section{Causal Receptivity Construct (Descriptive)}
\label{sec:app_receptivity}

We define the \emph{causal receptivity} of task type $\tau$ for optimizer $O$ as:
\begin{equation}
\text{receptivity}(\tau, O) = \sum_{f \in \text{fingerprint}(O)} \text{CATE}(f, \tau) \cdot \Delta f(O, \tau)
\end{equation}
where $\text{fingerprint}(O)$ is the set of features optimizer $O$ predominantly changes.
DSPy-MIPROv2 primarily changes Demos ($\overline{\Delta} = +0.974$) and Intrinsic\_load ($\overline{\Delta} = +0.811$).
Task-level Spearman correlation between mean CATE and optimizer success rate: $r = -0.866$, $p = 0.058$ ($n = 5$, borderline significant).
The negative sign suggests that spread and directionality of CATEs matters more than their mean.
A binary classifier (LOO-CV, $N = 20$ DSPy runs) achieved AUC~$= 0.260$, which is insufficient to support predictive claims.
This construct is reported as a \emph{descriptive summary} pending larger-scale interventional validation.

\section{SBERT Edit-Direction Sensitivity}
\label{sec:app_sbert}

PCA on SBERT embedding deltas (384-dim) of prompt pairs: 10 of 20 PCA components show sign reversals (spread~$> 0.05$) across task types.
PC7: commonsense~$+0.061\unc$, math~$-0.098\unc$, sequential~$+0.084\unc$ (spread~$= 0.181$).
These results are consistent with annotation-free robustness findings and suggest that the directional heterogeneity is detectable in semantic embedding space without any text-level feature engineering.
